# Supplementary material for: Robust Attack Graph Generation
Source: arXiv:2206.07776 source file (2022-06-15)
Supplement: Supplementary file 1 [file models.tex]

\section{Learned Models}
\label{app:models}
In Figure~\ref{fig:cptc-0}, the original learned model of the CPTC-2018 dataset can be seen. In Figure~\ref{fig:cptc-1}, the best iterated model of the CPTC-2018 dataset can be seen.  In Figures~\ref{fig:cptc-highlighted-0}~and~\ref{fig:cptc-highlighted-1}, the models are shown without sink states, and all edges with label ``vulnD|storage'' are highlighted red.

\begin{landscape}
 \begin{figure}[p]
  \centering
  \includegraphics[width=0.9\linewidth, keepaspectratio, height=\textwidth]{}
  \caption{The original model of the CPTC-2018 dataset, with sink states. It has an average normalised score of 0.66}
  \label{fig:cptc-0}
 \end{figure}
\end{landscape}

\clearpage

\begin{landscape}
 \begin{figure}[ht]
  \centering
  \includegraphics[width=0.95\linewidth, keepaspectratio, height=0.94\textwidth]{}
  \caption{The best iterated model of the CPTC-2018 dataset, with sink states. It has an average normalised score of 0.71.}
  \label{fig:cptc-1}
 \end{figure}
\end{landscape}

\clearpage

\begin{landscape}
 
\begin{figure}[htbp]
\floatconts
  {fig:cptc-highlighted}
  {\caption{Learned models of the CPTC-2018 dataset, without sink states. Edges with less than 10 occurrences are highlighted red. }}
  {\subfigure[Original model]{\label{fig:cptc-highlighted-0}%
      \includegraphics[height=0.9\textheight]{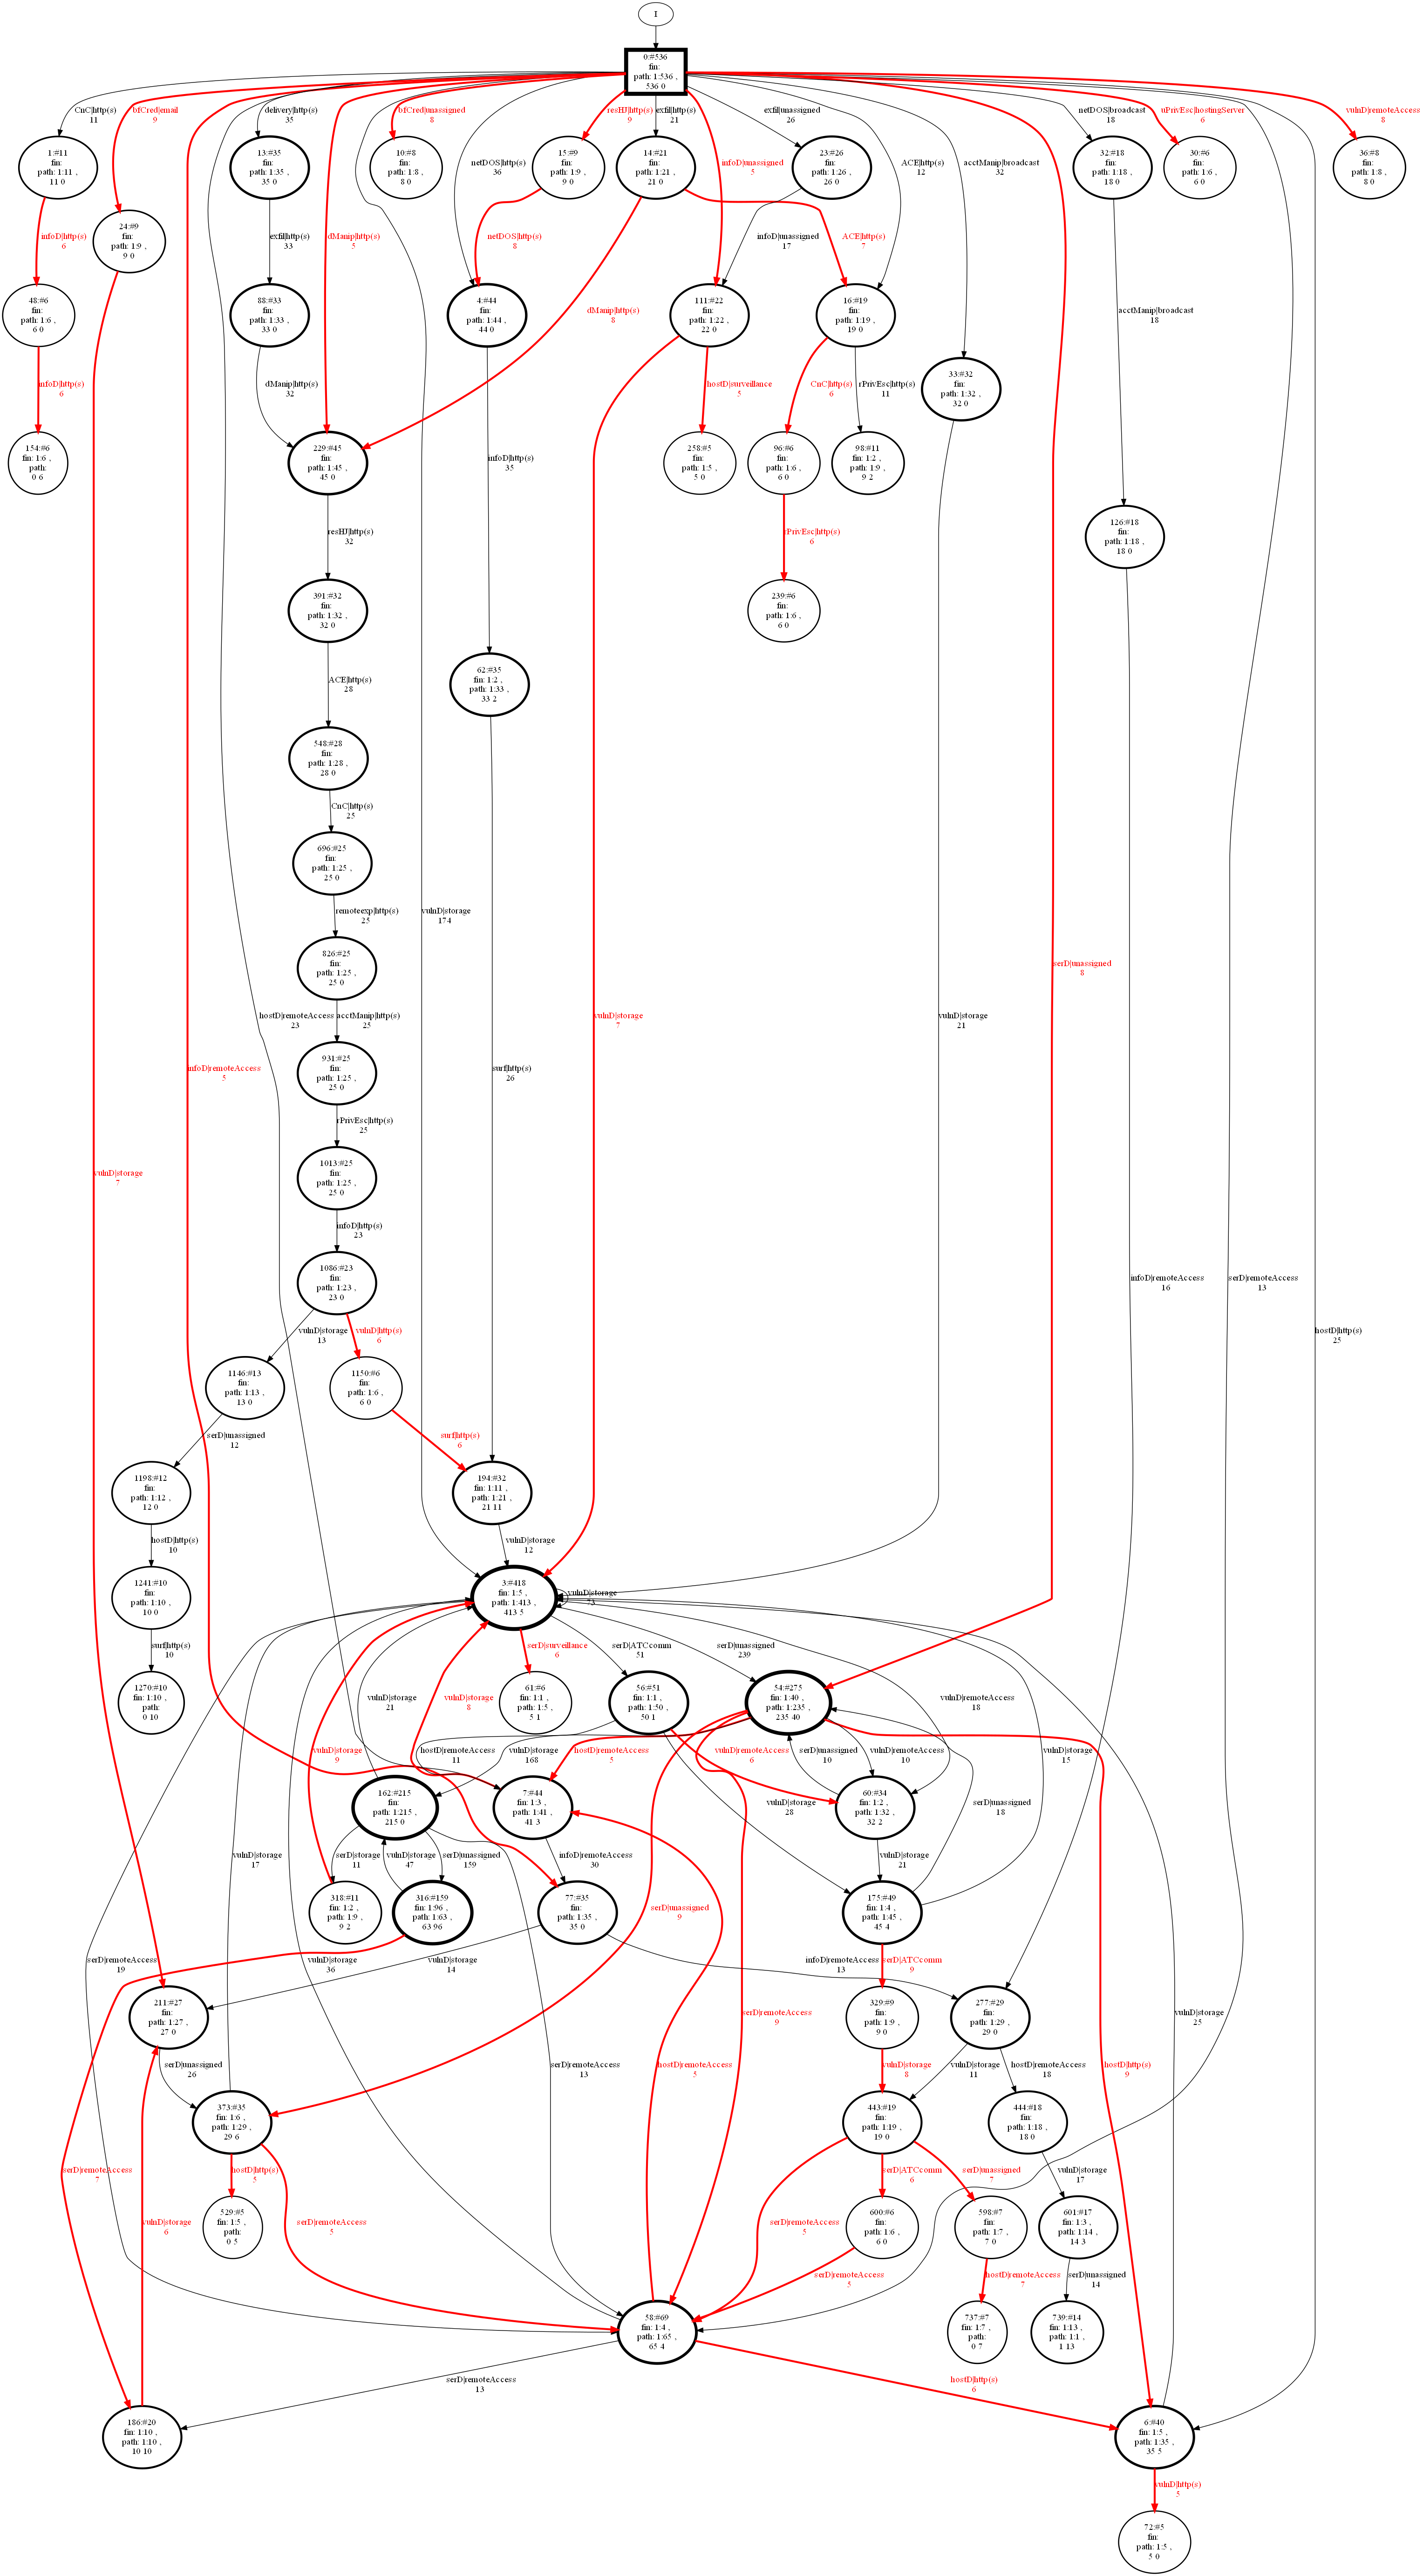}}%
    \qquad \qquad \qquad
    \subfigure[iterated \saat model]{\label{fig:cptc-highlighted-1}%
      \includegraphics[height=0.9\textheight]{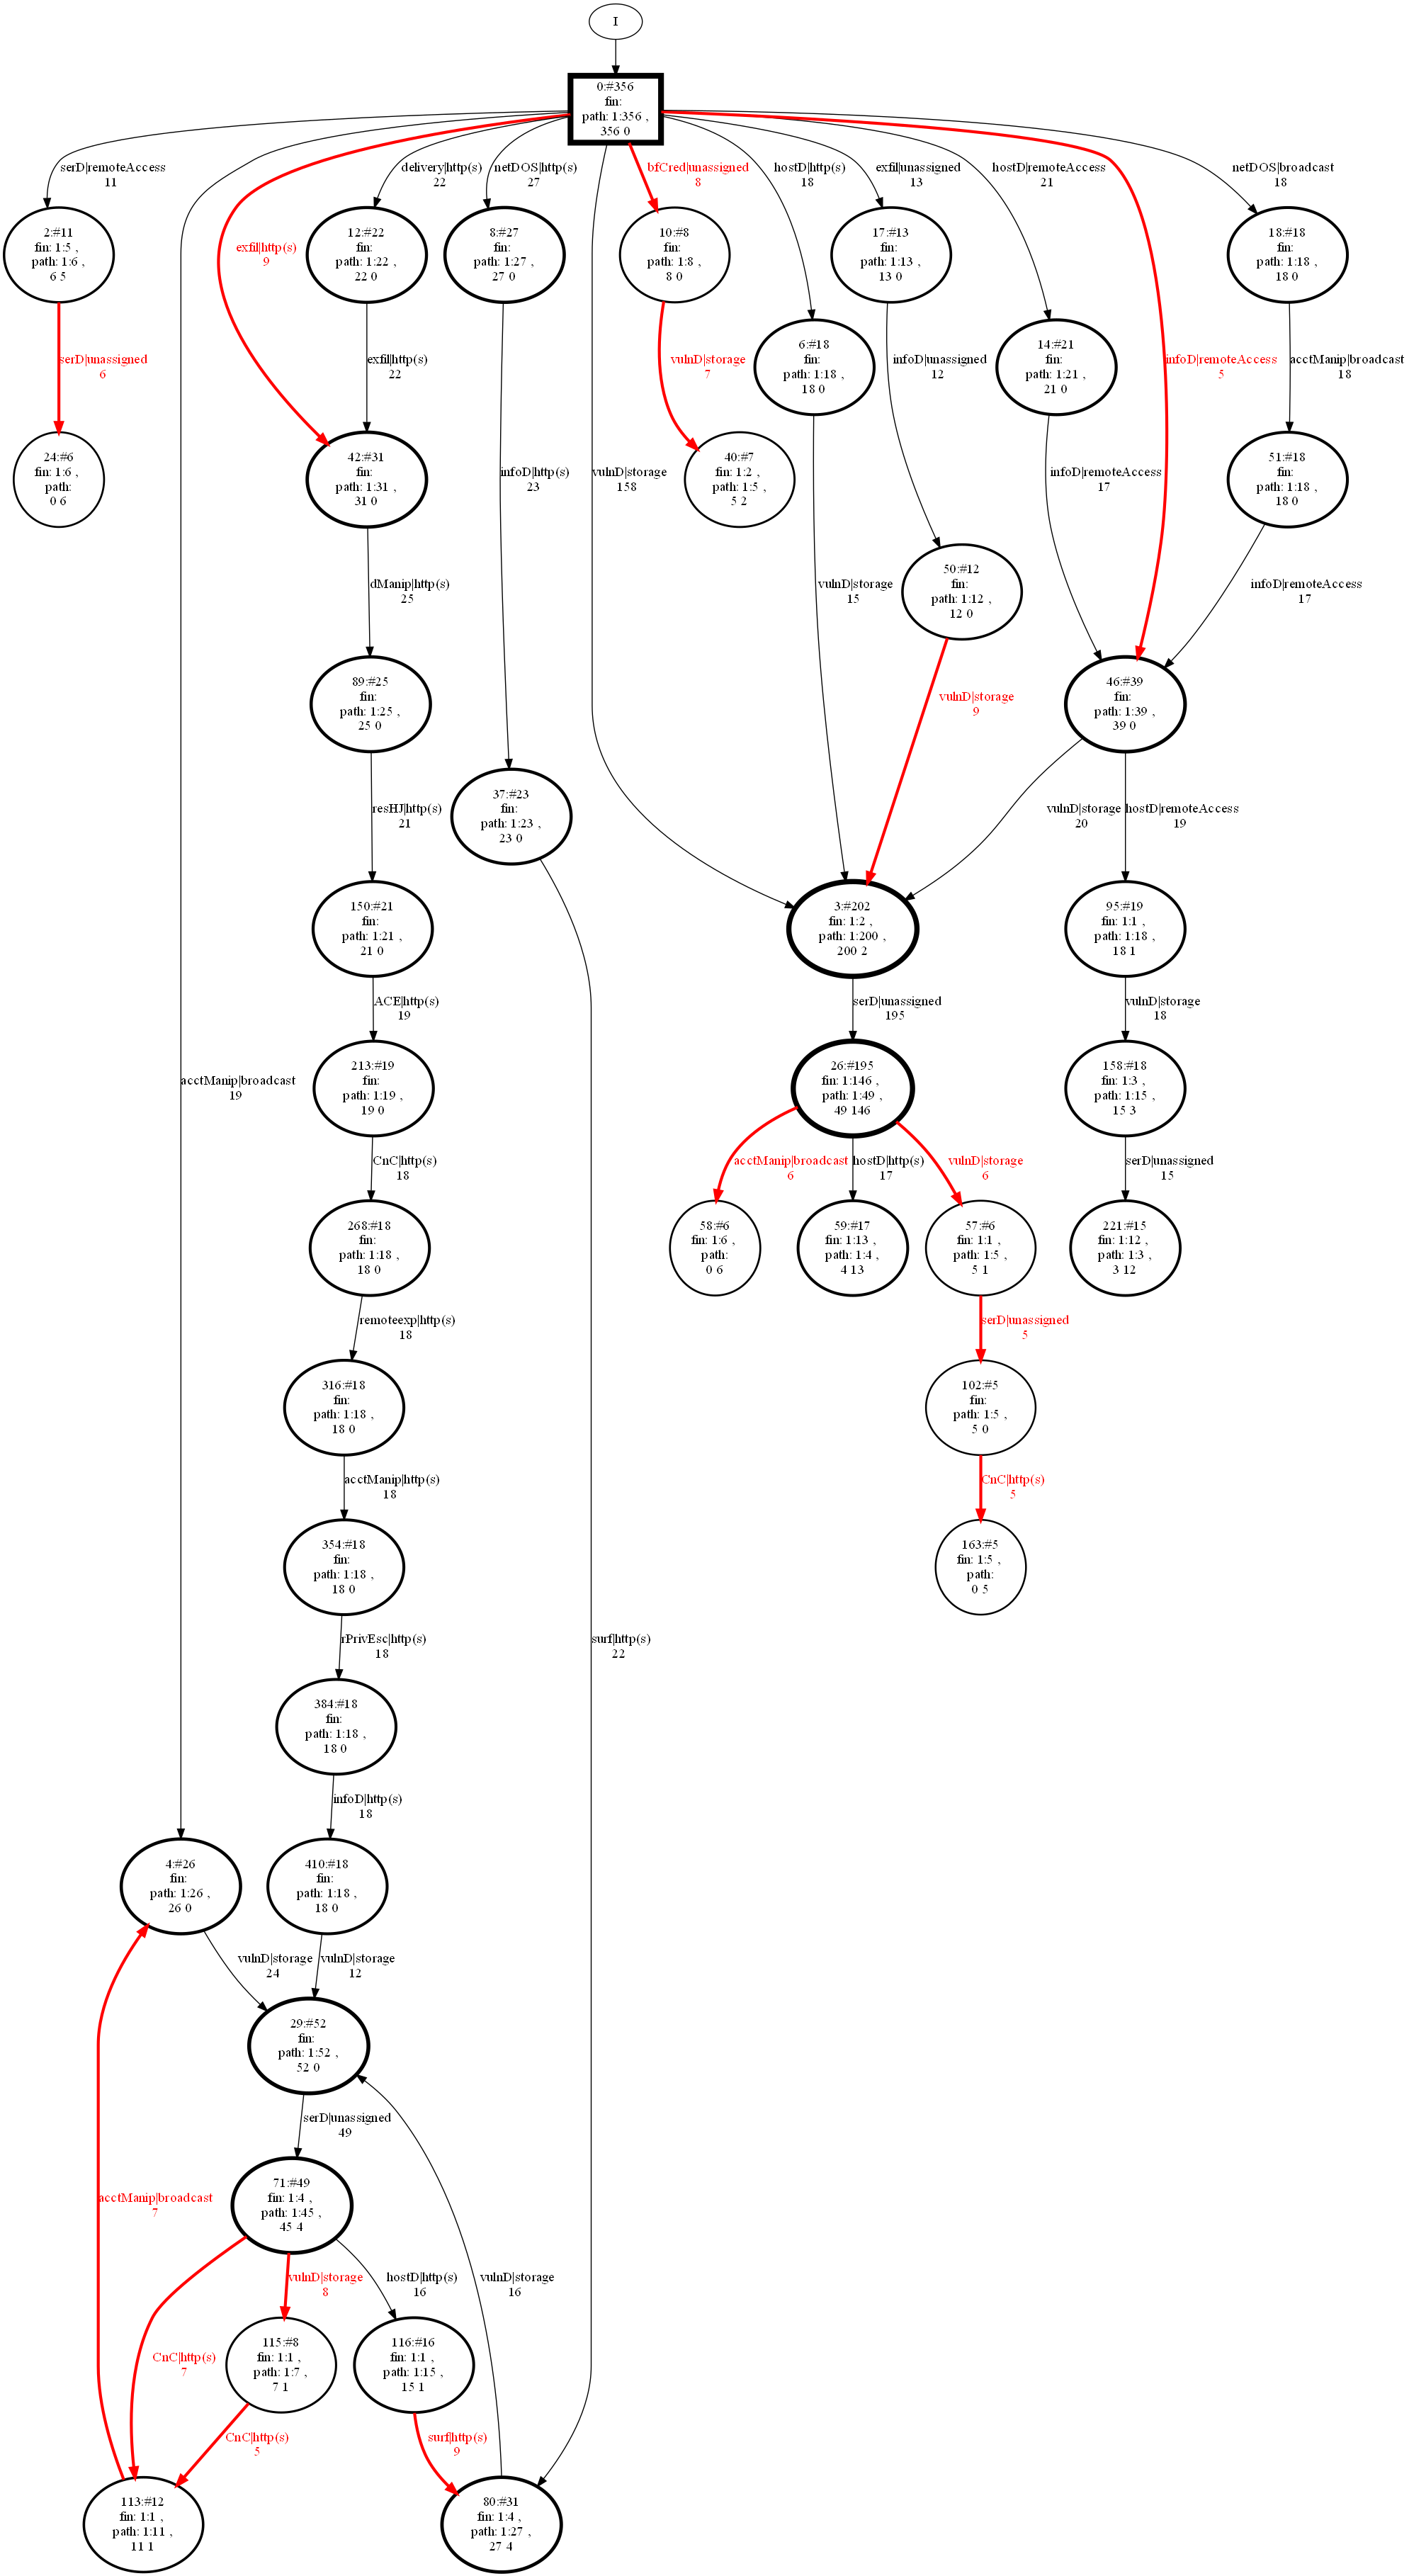}}
  }
\end{figure}
\end{landscape}
