# Supplementary material for: Robust Attack Graph Generation
Source: arXiv:2206.07776 source file (2022-06-15)
Supplement: Supplementary file 2 [file matched-sequence.tex]

\section{SAAT Backtracing Example and Algorithm}
\label{app:backtracking}

\begin{figure}[!ht]
\floatconts
  {fig:matched-sequence-cases}
  {\caption{Example situations to make a matched sequence. In both subfigures, the left part is transformed into the right part.}}
  {%
    \subfigure[A combination of a single skipped and added edge get transformed into an edge with the added edge's label (a).]{\label{fig:skipped_added}%
      \begin{tikzpicture}[scale=0.14]
            \tikzstyle{every node}+=[inner sep=0pt]
            \draw [black] (23.8,-13.7) circle (3);
            \draw [black] (23.8,-24.3) circle (3);
            \draw [black] (41.6,-13.7) circle (3);
            \draw [black] (41.6,-24.3) circle (3);
            \draw [black] (22.169,-21.806) arc (-158.19728:-201.80272:7.554);
            \fill [black] (22.17,-21.81) -- (22.34,-20.88) -- (21.41,-21.25);
            \draw (21.13,-19) node [left] {b (skipped)};
            \draw [black] (25.192,-16.34) arc (17.88374:-17.88374:8.661);
            \fill [black] (25.19,-21.66) -- (25.91,-21.05) -- (24.96,-20.74);
            \draw (26.11,-19) node [right] {a (added)};
            \draw [black] (41.6,-16.7) -- (41.6,-21.3);
            \draw (42.4,-19) node [right] {a};
            \fill [black] (41.6,-21.3) -- (42.1,-20.5) -- (41.1,-20.5);
        \end{tikzpicture}}%
    \qquad
    \subfigure[Multiple skipped edges.]{\label{fig:skipped_multiple}%
      \begin{tikzpicture}[scale=0.14]
            \tikzstyle{every node}+=[inner sep=0pt]
            \draw [black] (23.8,-13.7) circle (3);
            \draw [black] (23.8,-24.3) circle (3);
            \draw [black] (43.9,-13.7) circle (3);
            \draw [black] (43.9,-35.2) circle (3);
            \draw [black] (23.8,-35.2) circle (3);
            \draw [black] (43.9,-24.3) circle (3);
            \draw [black] (23.8,-16.7) -- (23.8,-21.3);
            \fill [black] (23.8,-21.3) -- (24.3,-20.5) -- (23.3,-20.5);
            \draw (23.3,-19) node [left] {b (skipped)};
            \draw [black] (25.437,-26.792) arc (22.28205:-22.28205:7.801);
            \fill [black] (25.44,-32.71) -- (26.2,-32.16) -- (25.28,-31.78);
            \draw (26.52,-29.75) node [right] {a (added)};
            \draw [black] (22.362,-32.584) arc (-161.04396:-198.95604:8.725);
            \fill [black] (22.36,-32.58) -- (22.57,-31.67) -- (21.63,-31.99);
            \draw (21.39,-29.75) node [left] {b (skipped)};
            \draw [black] (46.318,-15.463) arc (46.9166:-46.9166:12.305);
            \fill [black] (46.32,-33.44) -- (47.24,-33.26) -- (46.56,-32.53);
            \draw (51,-24.45) node [right] {a};
        \end{tikzpicture}}
  }
\end{figure}

%!TEX root = ../report.tex

\begin{fullwidth}[width=\linewidth+1cm]

\begin{algorithm2e}[H]
    \AlgorithmSetup

    \SetKw{Skipped}{SKIPPED}
    \SetKw{Added}{ADDED}
    \SetKw{Jump}{JUMP}
    \SetKw{source}{source}
    \SetKw{target}{target}
    \SetKw{name}{name}

    \KwIn{edges: $E$}
    \KwOut{matched sequence: $S$}
    \BlankLine

    $S = [ ]$\;
    $i = 0$\;
    \While{$i < \Len($E$)$}{
        $edge = E[i]$\;
        $i = i + 1$\;
        \If{$\type(edge) == \Skipped$} {
            $last\_edge = S[-1]$\;
            \While{$\type(E[i]) == \Skipped$} {
                $i = i + 1$\;
            }
            $new\_edge = (\source=last\_edge.\target, \target=E[i].\target, \name = E[i].\name)$\;
            $S.\Append(new\_edge)$\;
        }
        % \ElseIf{$\type(edge) == \Added$}{
        %     $S.\Append(edge)$\;
        % }
        \Else{
            $S.\Append(edge)$\;
        }
    }

    \caption{Create the \textit{matched} sequence from the alignment output}
    \label{code:fix-matched-sequence}
\end{algorithm2e}
\end{fullwidth}
